# Supplementary material for: Modeling Sustainable City Trips: Integrating CO2e Emissions, Popularity, and Seasonality into Tourism Recommender Systems
Source: arXiv:2403.18604 source file (2024-09-17)
Supplement: Supplementary file 1 [file appendix.tex]

\section{Appendix}
